# Supplementary material for: Deep learning enhanced initial model prediction in elastic FWI: application to marine streamer data
Source: arXiv:2501.12992 source file (2025-01-22)
Supplement: Supplementary file 1 [file ch8_appendice.tex]

\append{FWI workflow}
% \todo{The appendix is so short that i added it into the main text (see section DATASETS, subsection on training dataset)}  %% daniel: put into the main text

The open-source FWI code, which we use, allows us to customize the inversion workflow \citep{kohn2012,kohn_phdthesis} with many procedures (time filtering, gradient smoothing, time windowing, offset windowing, preconditioning, different misfit functions). These techniques allow mitigating the nonlinearity of the inversion process.

In the multi-stage FWI, which we perform, we aim to increase the upper frequency of band-pass time filtering with decreasing of smoothing factor for gradients in the FWI stages. In the workflows for FWI, we use Global Correlation norm misfit \citep{choi2012}. For creating the data for CNN we use the L2 norm.

%%% We also construct the workflow to perform FWI on the full-band data, having the spectrum starting from 2.5 Hz \figrefp{full_band_data_strategy_60}. We create it to get the reference FWI result on field marine data.

% In the workflows for FWI (Figures \figref{high_band_strategy_56}, \figref{full_band_data_strategy_60}) we use misfit LNORM=5, meaning Global Correlation norm misfit \citep{choi2012}. For creating the data for CNN we use L2 norm.

The open-source FWI code, which we use, allows us to customize the inversion workflow \citep{kohn2012,kohn_phdthesis} with many procedures (frequency filtering, gradient smoothing, time windowing, offset windowing, preconditioning, different misfit functions). These techniques provide opportunity to mitigate the nonlinearity of the inversion process.
For notations of FWI parameters presented in \figref{cnn_13_strategy_for_cnn_data}, \figref{high_band_strategy_56}, \figref{full_band_data_strategy_60} refer to the publications \citep{kohn2012,kohn_phdthesis}. The parameters we change in our FWI workflows are FC\_LOW, FC\_HIGH - lower and upper boundaries of time filtering; WD\_DAMP - gradient smoothing factor, LNORM - the type  of misfit.

We generate the high-wavenumber model updates for the CNN with the workflow presented in \figref{cnn_13_strategy_for_cnn_data}.

As soon as we intend to prove the quality of CNN-predicted initial models with further FWI on available data with a lack of low frequencies, we construct the workflow to invert this high-frequency data \figrefp{high_band_strategy_56}. We aim to increase the upper boundary of time filtering FC\_HIGH with decreasing of smoothing factor WD\_DAMP in the FWI stages.

We also construct the workflow to perform FWI on the full-band data, having the spectrum starting from 2.5 Hz \figrefp{full_band_data_strategy_60}. We create it to get the reference FWI result on field marine data.

In the workflows for FWI (Figures \figref{high_band_strategy_56}, \figref{full_band_data_strategy_60}) we use misfit LNORM=5, meaning Global Correlation norm misfit \citep{choi2012}. For creating the data for CNN we use L2 norm.

\fullplot{cnn_13_strategy_for_cnn_data}{width=2\columnwidth}{Workflow for creating the data for CNN.}
\fullplot{high_band_strategy_56}{width=2\columnwidth}{Workflow for high-frequency-band FWI on field data and synthetic data.}
\fullplot{full_band_data_strategy_60}{width=2\columnwidth}{Workflow for full-band FWI on field data.}

% To understand the spectrum of high-frequency data, which we deal with, please refer to \figrefp{marm_first_shot_high_pass_filtering2}d. It ranges from 5~Hz to 14~Hz.
